# Supplementary material for: Evidence-Based Intelligent Diagnostic and Therapeutic Visualization System with Large Language Models: Multi-Turn Interaction and Multimodal Treatment Plan Generation
Source: arXiv:2606.06869 source file (2026-08-28)
Supplement: Supplementary file 1 [file si.tex]

\documentclass[12pt]{article}
\usepackage[utf8]{inputenc}
\usepackage{graphicx}
\usepackage{amsmath}
\usepackage{booktabs}
\usepackage{hyperref}
\usepackage{listings}
\usepackage{tcolorbox}
\tcbuselibrary{listings,breakable}
\newtcblisting{promptbox}[1]{
  breakable,
  colframe=gray,
  colback=gray!5!white,
  coltitle=white,
  coltext=black,
  fonttitle=\bfseries,
  title={#1},
  boxrule=1pt,
  arc=2mm,
  width=\linewidth,
  left=3pt,
  right=3pt,
  top=3pt,
  bottom=3pt,
  listing only,
  listing options={
    basicstyle=\fontsize{8.5pt}{10pt}\selectfont\ttfamily,
    breaklines=true,
    breakatwhitespace=true,
    columns=fullflexible,
    keepspaces=true,
    showstringspaces=false
  }
}
\usepackage[left=2.5cm,right=2.5cm,top=2.5cm,bottom=2.5cm]{geometry}

% SI reference numbering: prefix all references with "S" to avoid
% conflicting with main paper's [1]-[26] numbering
\makeatletter
% Bibliography list labels: [1] -> [S1]
\renewcommand{\@biblabel}[1]{[S#1]}
% In-text citations: intercept \bibcite to prepend S to each number,
% so \cite produces [S1] instead of [1] (works with multi-cites too)
\let\originalbibcite\bibcite
\renewcommand{\bibcite}[2]{\originalbibcite{#1}{S#2}}
\makeatother

\title{Supporting Information\\
\large AI-Assisted Diagnostic System for Traditional Chinese Medicine}
\date{}

\begin{document}
\maketitle
\tableofcontents
\newpage

\section{S1: Related Work --- Detailed Literature Review}
\label{sec:si-related-work}

\subsection{AI-Assisted TCM Diagnostic Systems}

AI-assisted diagnostic systems have evolved from rule-driven to data-driven approaches. Survey literature has systematically reviewed the development and challenges of large language models in healthcare~\cite{7,14,8}. In recent years, the emergence of LLMs has given rise to a new generation of intelligent TCM systems: the knowledge-tuning approach fine-tunes LLMs with structured TCM knowledge bases to improve reliability~\cite{60}; BianQue enhances multi-turn consultation capabilities through hybrid instruction fine-tuning~\cite{61}; HuatuoGPT-Vision explores injecting medical visual knowledge into multimodal LLMs~\cite{62}.

However, existing systems have two shortcomings: first, most adopt a single-turn interaction mode without multi-turn information-gathering mechanisms that simulate real consultations; second, diagnostic reasoning is opaque to users, with no system-level design for presenting reasoning paths visually. Our system attempts to fill this gap through a knowledge-graph-driven multi-turn dialogue framework and progressive reasoning visualization.

\subsection{Knowledge Graph Visualization and Medical Interaction}

Knowledge graph visualization serves as a critical link between structured knowledge and human cognition. Prior work has conducted systematic performance analyses of large-scale knowledge graph visualization methods~\cite{24}, noting that node-link diagrams offer intuitive advantages for expressing entity relationships but face readability challenges at scale. Controlled experiments~\cite{34} have further evaluated the cognitive efficiency of different graph representations, providing empirical evidence for interactive graph design. On the task-modeling front, a multi-level abstract task taxonomy~\cite{33} supplies a theoretical framework for understanding user interaction patterns with visualization systems.

In the healthcare domain, KNOWNET~\cite{35} is a representative system combining knowledge graphs with LLMs for health information retrieval, supporting user exploration of medical knowledge through progressive graph visualization and entity neighborhood browsing. Sukhwal et al.~\cite{25} proposed a joint LLM-KG system for disease question answering, demonstrating the potential of knowledge graphs to constrain generated content. Interactive visual analytics frameworks have also shown the ability to guide users through complex relationships in biomedical data analysis~\cite{56}.

However, knowledge graph visualization in these works largely functions as a standalone knowledge browsing tool, where users explore the graph freely, decoupled from the diagnostic decision process. Our system deeply embeds knowledge graph visualization within the diagnostic workflow, producing case-specific subgraphs that update progressively with each consultation turn, making the evolution of reasoning paths transparent and traceable.

\subsection{Multimodal Medical Information Presentation}

The value of multimodal information presentation in medical education and patient communication is widely recognized. Related research~\cite{9} has explored the potential of multimodal LLMs based on individual-level data for health management; a survey~\cite{30} systematically reviewed methods for integrating knowledge graphs with multimodal learning, identifying cross-modal knowledge alignment as key to improving model understanding. In medical visualization, three-dimensional anatomical visualization has been applied to meridian system modeling~\cite{63}, while discussions on AI-generated anatomical images~\cite{47} have revealed both the potential and limitations of this direction.

Existing systems remain limited in multimodal presentation of treatment plans: text-dominant treatment recommendations lack intuitiveness, and spatial information such as acupoint localization is difficult to convey effectively through planar media. Our system integrates AI-generated treatment illustrations and a three-dimensional acupoint model, providing a fused text, image, and 3D interactive experience during treatment presentation to improve patient comprehension of treatment plans.

\subsection{LLM Hallucination Mitigation and Knowledge Grounding}

Hallucination in large language models is one of the core obstacles limiting their clinical application. Pal et al.~\cite{13} proposed Med-HALT, a hallucination testing benchmark for the medical domain, systematically quantifying fabrication and misleading behaviors in LLM medical reasoning. Huang et al.~\cite{44} provided a comprehensive survey of LLM hallucinations covering principles, taxonomy, and challenges. Kim et al.~\cite{45} further analyzed the potential impact of foundation model hallucinations on medical decision-making.

Mainstream approaches to hallucination mitigation follow two paths: RAG~\cite{29} and external knowledge base augmentation~\cite{68}. Most methods, however, treat the knowledge graph merely as a retrieval source to supplement LLM context. Our system adopts a different strategy: the knowledge graph serves not only as a retrieval resource but as a structural constraint. By defining the candidate diagnostic space and driving symptom selection strategies through the KG, the diagnostic reasoning process remains bounded within the evidence frontier delineated by the graph structure. This ``scaffold'' approach to knowledge grounding complements post-hoc knowledge retrieval verification.

\subsection{Comparison with Representative Systems}

To clearly position our system's design space, Table~\ref{tab:comparison} compares representative TCM and health intelligence systems across six dimensions. Each system demonstrates its own strengths and emphases under different design objectives.

\begin{table}[htbp]
\centering
\caption{Comparison of representative TCM intelligent systems}\label{tab:comparison}
\resizebox{\linewidth}{!}{%
\begin{tabular}{lcccc}
\toprule
Aspect & KNOWNET\cite{35} & BianQue\cite{61} & Knowledge-tuning\cite{60} & Ours \\
\midrule
Diagnostic approach & KG-validated LLM output & LLM multi-turn consultation & KG-finetuned LLM & KG-driven info-theoretic consultation \\
Visualization & Progressive graph & None & None & Progressive KG \\
Interaction mode & User-driven browsing & Multi-turn dialogue & Single-turn QA & System-initiated questioning \\
Knowledge representation & External KG mapping & Finetuned LLM & Structured KB & KG+LLM hybrid \\
Treatment visualization & None & None & None & AI illustrations + 3D acupoints \\
\bottomrule
\end{tabular}
}
\end{table}

The core strength of KNOWNET~\cite{35} lies in its post-hoc verification strategy, which suits health information retrieval scenarios. BianQue~\cite{61} excels in multi-turn dialogue capability but lacks visual support for reasoning processes. The knowledge-tuning approach~\cite{60} focuses on enhancing LLM domain reliability through knowledge base augmentation.

Our system is distinguished by three design choices: (1) elevating the knowledge graph from a verification tool to the structural backbone of the diagnostic workflow, driving dynamic candidate space updates and information-theoretically guided symptom selection; (2) making multi-turn reasoning transparent through progressive subgraph visualization; (3) providing multimodal output that includes a three-dimensional acupoint model and AI-generated illustrations during treatment presentation. These design choices are not uniformly superior to other systems but represent a system-level integration targeting two specific goals: diagnostic process transparency and treatment plan intuitiveness.

\section{S2: Implementation Details}
\label{sec:si-implementation}

\subsection{Technical Architecture}\label{subsec:tech-arch}

The system is implemented as a three-tier architecture with separated front-end and back-end. The front-end is built with Next.js~15 and React~19 as a single-page application providing a responsive interactive interface; the back-end uses the Flask framework to provide RESTful API services, hosting the core computational logic of diagnostic reasoning; the data layer uses a Neo4j graph database to store the knowledge graph (241 syndrome types, 1,263 symptoms, 2,485 relationships) and accesses the large language model service through the Gemini~3.1~Pro API (Google), with BGE-M3 as the semantic embedding model. The system runs on Python~3.11 and Node.js~18+, with support for Docker containerized deployment.

\subsection{Four-Layer Symptom Matching Mechanism}\label{subsec:symptom-matching}

As described in the main paper's System Design section, the system needs to accurately align user natural language symptom descriptions to standardized entities in the knowledge graph. To balance matching precision and robustness, we designed a four-layer progressive matching mechanism, executed in order from highest to lowest matching precision:

\textbf{Layer 1: Exact matching}: The system performs case-insensitive string comparison between user input and KG symptom entity labels, returning an immediate match result upon exact correspondence.

\textbf{Layer 2: Semantic vector matching}: When exact matching fails, the BGE-M3 embedding model computes the cosine similarity between user symptom mention $\nu$ and KG symptom entities $\xi \in \Omega$:
\begin{equation}\label{eq:sim}
\mathrm{sim}(\nu, \xi) = \frac{\mathbf{e}(\nu) \cdot \mathbf{e}(\xi)}{\|\mathbf{e}(\nu)\| \cdot \|\mathbf{e}(\xi)\|}
\end{equation}
where $\mathbf{e}(\cdot)$ denotes the BGE-M3 embedding function. The match is accepted when the highest similarity exceeds the threshold $\delta$.

\textbf{Layer 3: Fuzzy matching}: For spelling variants and abbreviations in user input, the system uses the rapidfuzz library's \texttt{token\_set\_ratio} algorithm to compute fuzzy similarity, with a threshold of $\tau$.

\textbf{Layer 4: LLM verification}: For ambiguous cases that the first three layers cannot resolve, a fast LLM is invoked to output verification results in structured JSON format, serving as the final fallback strategy.

Combining the four layers above, the symptom matching function is defined as:
\begin{equation}\label{eq:match}
\mathrm{match}(\nu) = \begin{cases}
\xi & \text{if } \nu = \xi \text{ (exact match)} \\
\arg\max_{\xi} \mathrm{sim}(\nu, \xi) & \text{if } \mathrm{sim} \geq \delta \\
\arg\max_{\xi} \mathrm{fuzz}(\nu, \xi) & \text{if } \mathrm{fuzz} \geq \tau \\
\mathrm{LLM}(\nu, \Omega) & \text{otherwise}
\end{cases}
\end{equation}
This cascading mechanism ensures that common cases are resolved quickly through efficient string and vector operations, invoking the more costly LLM service only when necessary.

\subsection{Information Gain-Driven Follow-up Selection}\label{subsec:ig-question}

At each interaction round, the system selects the most discriminative symptom subset $Q_t$ from the unasked symptom space for follow-up, aiming to maximally reduce the diagnostic uncertainty of the candidate syndrome type set $\mathcal{Y}_t$. We adopt an information gain-driven weighted utility function:
\begin{equation}\label{eq:utility}
U(Q_t) = \alpha \cdot \mathrm{IG}(Q_t; \mathcal{Y}_t) - \beta \cdot \mathrm{Redundancy}(Q_t) + \gamma \cdot \mathrm{Coverage}(Q_t)
\end{equation}
where $\mathrm{IG}$ measures the entropy reduction in the candidate space after asking $Q_t$, reflecting the information value of the question; $\mathrm{Redundancy}$ penalizes highly correlated redundant questions through mutual information between symptoms; and $\mathrm{Coverage}$ encourages selecting symptom combinations that cover more discriminative features across candidate syndrome types. The parameters $\alpha$, $\beta$, and $\gamma$ control the relative weights of the three terms.

Since question selection is inherently a combinatorial optimization problem and exhaustive search is infeasible when the candidate symptom space is large, the system uses a genetic algorithm for approximate optimization, with the utility function $U(Q_t)$ as the fitness function.

\subsection{Engineering Optimizations}\label{subsec:engineering}

To ensure responsive performance in production deployment, we implemented the following engineering optimizations:

\textbf{KG warm-up cache}: At application startup, the system loads all syndrome type-symptom mappings from Neo4j into memory in a single batch, constructing a module-level cache. Subsequent requests read directly from memory, avoiding repeated graph database queries and significantly reducing query latency during diagnostic reasoning.

\textbf{Embedding vector cache}: BGE-M3 embedding vectors for all symptom names in the KG are precomputed, using the SHA-256 hash of the symptom vocabulary as the cache invalidation key, with the embedding matrix persisted to disk. When the KG content has not changed, the system loads the cached vector matrix at startup, avoiding redundant GPU computation overhead.

\textbf{Parallel computation}: In batch embedding computation scenarios, the system uses \texttt{ThreadPoolExecutor} to execute concurrent embedding requests for multiple symptom terms, reducing overall response time when matching multiple symptoms simultaneously.

\textbf{LLM structured output repair}: To address the instability of LLM output formats, we built a three-stage JSON parsing pipeline: first attempting direct parsing, then extracting JSON fragments from code fences via regular expressions, and finally having the LLM self-repair and regenerate. This pipeline effectively handles common output anomalies such as Markdown fence wrapping and appended explanatory text.

\textbf{Skeleton screen loading}: The front-end displays skeleton screen placeholders while awaiting API responses, maintaining stable interface layout, preserving perceived responsiveness, and avoiding interface flickering caused by network latency.

\subsection{Knowledge Graph Visualization Implementation}\label{subsec:kg-viz}

The system's knowledge graph visualization is built on the ECharts force-directed graph, embedded in the front-end right panel via an iframe. The visualization module responds to diagnostic progress changes in real time: whenever a new symptom is confirmed or candidate syndrome types are updated, the graph automatically refreshes to dynamically display the current case-specific subgraph. Nodes use a categorical color scheme: symptom nodes in red, syndrome type nodes in green, and the currently selected node highlighted, helping users quickly distinguish different entity types and their associations.

During the treatment plan presentation phase, the system integrates the 3D acupoint model, supporting rotation and zoom interactions, with the ability to highlight acupoints relevant to the current treatment plan. Additionally, symptom keywords in the chat interface are highlighted in yellow, enabling users to intuitively identify symptoms captured by the system during conversation.

\section{S3: Case Study --- Detailed Walkthrough}
\label{sec:si-case-study}

To illustrate the system's diagnostic workflow concretely, we present a representative case involving a patient with dizziness, insomnia, and dry mouth,
walking through the complete four-module interaction process described in Section~2.2 of the main paper.

\paragraph{Module 1: Symptom Input and Initial Graph Construction}
The patient describes in natural language: ``I've been getting dizzy a lot recently, I can't sleep well at night, and my mouth is dry when I wake up.''
Through the four-layer matching mechanism (see Section~2.2), the system extracts and standardizes three core symptoms: \textit{dizziness}, \textit{insomnia}, and \textit{dry mouth}.
The system then queries the Neo4j knowledge graph and constructs an initial subgraph containing these symptoms, identifying 5--6 candidate syndrome patterns,
including Liver-Kidney Yin Deficiency, Qi-Blood Deficiency, and Heart-Kidney Disharmony.
As shown in Figure~6 in the main paper, the knowledge graph visualization at this stage highlights the association paths between confirmed symptom nodes and candidate syndrome patterns,
allowing users to observe the composition of the initial diagnostic space intuitively.

\paragraph{Module 2: Multi-Round Follow-Up and Dynamic Graph Updates}
Based on information gain analysis, the system selects the symptom features most valuable for differentiating among the current candidate syndrome patterns
and directly lists candidate symptoms for user confirmation: ``Do you have any of the following symptoms: red tongue with thin coating, thin and rapid pulse, palpitations?''
After the user confirms present symptoms, unmentioned symptoms are treated as implicitly denied.
Over two rounds of interaction, supplementary information is obtained: red tongue with thin coating, thin and rapid pulse.
The system updates the knowledge graph accordingly: candidate syndrome patterns that do not match the newly confirmed symptoms receive lower match scores and gradually fade,
narrowing the candidate space from 5--6 to 3. As shown in Figure~4 in the main paper,
the progressive changes in the graph after each interaction round keep the diagnostic reasoning process transparent and traceable.

\paragraph{Module 3: Multi-Layer Matching and Syndrome Ranking}
The system performs four-layer progressive matching and ranks candidate syndrome patterns by the number of confirmed symptoms matched:
(1)~\textbf{Liver-Kidney Yin Deficiency}, matching 5/6 symptoms: dizziness, insomnia, dry mouth, red tongue with thin coating, and thin and rapid pulse together form the characteristic symptom cluster for this syndrome pattern;
(2)~\textbf{Qi-Blood Deficiency}, matching 3/5 symptoms: dizziness and insomnia match, but tongue and pulse characteristics do not fully align;
(3)~\textbf{Heart-Kidney Disharmony}, matching 2/5 symptoms: insomnia and dry mouth are relevant, but key differentiating symptoms such as palpitations are absent.
As shown in Figure~7 in the main paper, the ranked results include the supporting symptom list and match degree for each candidate syndrome pattern,
providing users with traceable diagnostic evidence.

\paragraph{Module 4: Multimodal Treatment Plan Generation}
Based on the top-ranked Liver-Kidney Yin Deficiency syndrome pattern, the system generates a comprehensive treatment plan:
the herbal formula Liuwei Dihuang Wan (with modifications), supplemented by dietary recommendations (yin-nourishing ingredients such as goji berry and Chinese yam) and lifestyle guidance.
Acupoint recommendations include Taixi and Sanyinjiao, displayed with spatial positioning on a 3D bronze figure model (as shown in Figure~9 in the main paper),
which users can rotate and zoom to precisely locate acupoint positions.
AI-generated treatment illustrations (as shown in Figure~8 in the main paper) present dietary plans visually,
lowering the cognitive barrier for non-specialist users to understand treatment information.
The complete treatment advice interface (as shown in Figure~10 in the main paper) integrates these multimodal elements into a structured diagnostic report.
This module enhances treatment plan comprehensibility through multimodal integration.

\section{S4: Statistical Methods}
\label{sec:si-statistics}

\subsection{Case Selection}

Evaluation cases were drawn from a dataset of 160 de-identified TCM electronic medical records (CEMRs).
We adopted a \textbf{stratified random sampling by syndrome type} strategy (random seed $= 42$), using syndrome type labels as the stratification variable,
allocating quotas proportionally to each syndrome type's representation in the population, ensuring each syndrome type received at least 1 sampling quota.
A total of 30 test cases were selected, covering no fewer than 5 distinct syndrome types, ensuring the evaluation sample's representativeness of syndrome type diversity.
For the LLM-as-a-Judge experiments, RQ2 and RQ3.1 each used all 30 cases, while RQ3.2 used 25 of these (excluding cases where the back-end treatment recommendation API did not return references).

\subsection{Judge Model Configuration}

The judge used the Claude Sonnet~4.5 model (Anthropic), with \texttt{temperature=0} to ensure deterministic outputs. To avoid same-source bias, the judge model was deliberately selected from a different vendor than the system's main model and patient simulator (both from the Google family).
For each evaluation dimension, we designed natural language judging criteria,
and the judge model independently scored on a 1--5 Likert scale according to these criteria, where 1 indicates ``very poor'' and 5 indicates ``very good.''
The judge model was required to output scores and reasoning for each dimension in structured JSON format,
with outputs validated through a three-stage JSON parsing pipeline (direct parsing $\rightarrow$ regex extraction $\rightarrow$ pattern matching),
ensuring dimension completeness: if a dimension was missing, the system automatically retried (up to 2 times) and, upon exhausting retries, filled in the default minimum score.

\subsection{Statistical Analysis Methods}

Given the small paired sample size ($n \leq 30$) and ordinal nature of the score data,
we used the \textbf{Wilcoxon signed-rank test} (two-sided) for between-condition difference testing,
with the significance level set at $\alpha = 0.05$.
To address the multiple comparison problem arising from simultaneous testing across dimensions,
we applied \textbf{Benjamini--Hochberg FDR correction} to all $p$-values.
For effect sizes, RQ2 and RQ3.2 used \textbf{Cohen's $d$} (paired samples) to measure the practical significance of between-group differences;
RQ3.1, due to reverse-scored dimensions producing many zero values in the differences,
used \textbf{rank-biserial $r$} as the effect size measure,
which is computed directly from the Wilcoxon statistic ($r = 1 - 2W / n(n+1)$) and is more robust to zero values.

\subsection{RQ2: Trust Evaluation with KG Augmentation}

RQ2 assessed whether KG visualization improves patient trust in diagnostic results.
The experiment used a paired design: for each case, a patient simulator based on the Gemini~3~Flash model (Google) first completed the full multi-round consultation interaction with the system (up to 5 rounds),
obtaining diagnostic results and knowledge graph data;
the judge model then evaluated the same consultation process under two conditions, \textit{with KG visualization} and \textit{without KG visualization},
from the patient's perspective.
The evaluation covered 5 trust dimensions: \textbf{diagnostic transparency} (whether patients can understand how the diagnosis was derived),
\textbf{evidence traceability} (whether the associations between symptoms and diagnoses are visible and verifiable),
\textbf{reasoning confidence} (the patient's confidence in the system's reasoning process),
\textbf{information completeness} (whether the consultation provided sufficient information for judgment), and
\textbf{overall trust level} (whether the patient trusts and accepts the diagnostic results).
Under the KG condition, the judge model was provided with a complete description of the interactive KG,
including symptom-syndrome connections, node interaction features, and etiology and pathogenesis information of syndrome types.

\subsection{RQ3.1: Cognitive Load Evaluation of Multimodal Treatment Plans}

RQ3.1 assessed whether structured multimodal treatment plans can reduce cognitive load for non-expert users.
The judge model was assigned the role of an \textit{ordinary user with only middle school education, no medical background, and residing in a rural area},
to simulate the knowledge level and information comprehension ability of the target audience.
\textbf{Plan A} was the system-generated plain-text treatment recommendation in its original form;
\textbf{Plan B} restructured Plan A into a structured format,
integrating step-by-step operational guides, herbal ingredient identification images (AI-generated, up to 2 per case),
and text descriptions of 3D acupoint models and demonstration videos.
The evaluation covered 5 cognitive dimensions: \textbf{language comprehensibility}, \textbf{preparation clarity},
\textbf{acupoint localizability}, \textbf{action execution confidence}, and \textbf{overall cognitive load}.
The ``overall cognitive load'' dimension used \textbf{reverse scoring}:
in the original scoring, 1 indicates ``very easy'' and 5 indicates ``very effortful,''
and during analysis this was converted to $6 - \text{original score}$,
so that all dimensions share a consistent scoring direction (higher scores indicate lower cognitive load, i.e., better user experience).
This reverse scoring design ensures comparability and the validity of aggregate analysis between this dimension and the four positively scored dimensions.

\subsection{RQ3.2: Evidence Credibility Evaluation of References}

RQ3.2 assessed whether appending references to treatment recommendations improves the evidence credibility of the information.
The experiment likewise used a paired design: under the \textit{with references} condition,
the judge model was provided with the full treatment recommendation text and the system-retrieved reference list
(including titles, URLs, and abstract snippets);
under the \textit{without references} condition, only the treatment recommendation text was provided.
To enhance evaluation rigor, the system used a URL scraping tool to retrieve the actual page content of each reference link
(truncated to the first 2,000 characters), providing this to the judge model
so that it could verify the \textbf{accessibility} and \textbf{content relevance} of cited sources.
The evaluation covered 5 evidence dimensions: \textbf{source credibility}, \textbf{evidence verifiability},
\textbf{information confidence}, \textbf{comprehension support}, and \textbf{overall evidence quality}.

\section{S5: Evaluation Prompts}
\label{sec:si-eval-prompts}

This section documents the complete set of LLM-as-Judge prompts used in the evaluation pipeline described in Section~\ref{sec:si-statistics}. For prompt subsets tied to specific research questions, the RQ identifiers (e.g., RQ2, RQ3.1, RQ3.2) correspond to the main paper's research questions.

\subsection{Patient Simulator Prompts}
The patient simulator (based on Gemini 3 Flash) plays the role of a simulated patient during multi-round diagnostic consultations. It translates Chinese medical terms from its assigned clinical profile into English symptom terms.

\begin{promptbox}{Listing 1: System prompt.}
You are a simulated patient reporting symptoms to a doctor. Your
medical profile may contain Chinese medical terms. ALWAYS translate
Chinese terms into concise English medical nouns (e.g. headache,
insomnia, palpitations, pale complexion, cold extremities). Output
ONLY symptom terms separated by commas. Never write full sentences,
narratives, or explanations. Never invent symptoms outside your
medical profile.
\end{promptbox}

\begin{promptbox}{Listing 2: Initial symptom description prompt.}
Translate the following symptoms into English medical terms and
list them as a comma-separated list. Output ONLY the terms.

Symptoms: {CLINICAL_FEATURES}
English terms:
\end{promptbox}

\begin{promptbox}{Listing 3: Follow-up response prompt.}
The doctor asks about specific symptoms. Check each against your
clinical profile.

Your profile: {CLINICAL_FEATURES}
Asked symptoms: {ASKED_SYMPTOMS}

Output ONLY the symptoms from the asked list that match your
profile. List them as comma-separated English medical terms. Do NOT
mention symptoms you don't have -- just omit them entirely. If none
match your profile, output exactly: none
\end{promptbox}

\subsection{Trust Evaluation Prompts (RQ2)}
The trust evaluation assesses whether knowledge graph visualization improves patient trust in diagnostic results (corresponding to RQ2 in the main paper). The judge model evaluates the consultation under two conditions: with and without KG visualization.

\begin{promptbox}{Listing 4: Judge system prompt.}
You are evaluating a Traditional Chinese Medicine (TCM) diagnostic
consultation from the patient's perspective. The patient used a
web-based TCM diagnostic application that:
1. Lets the patient describe symptoms in free text
2. Extracts medical terms via NLP from the description
3. Queries a TCM Knowledge Graph to find candidate syndromes
4. Asks targeted follow-up questions derived from KG relationships
5. Presents a ranked diagnosis with confidence scores
6. (With KG condition only) Shows an interactive knowledge graph
   visualization that maps the patient's symptoms to candidate
   syndromes visually

IMPORTANT EVALUATION CONTEXT:
- This is a structured diagnostic system, not a conversational
  chatbot
- The system uses medical knowledge graph traversal to generate
  follow-up questions
- Follow-up questions target specific symptoms that differentiate
  between candidate syndromes
- The consultation record below describes the patient-facing
  experience as it appears in the application interface
- When KG visualization is present, the patient can interactively
  explore symptom-syndrome connections, hover for detailed
  explanations, and visually verify the diagnostic reasoning

Evaluate how TRUSTWORTHY and CREDIBLE the diagnostic process
appears to the patient. Focus on whether the patient can
understand, verify, and ultimately trust the reasoning behind
the diagnosis.

Use only the provided evidence and return valid JSON.
\end{promptbox}

\begin{promptbox}{Listing 5: Judge user prompt template.}
Case ID: {CASE_ID}
Reference syndrome label: {SYNDROME}

You are a patient who just completed this diagnostic consultation
in a web-based TCM diagnostic application.

{CONSULTATION_TRANSCRIPT}

{CONDITION_DESCRIPTION}

Evaluate this consultation strictly from the patient's perspective.
Consider: Can you understand WHY this diagnosis was reached? Can
you verify the reasoning? Do you trust the result?

Use a 1-5 Likert score for each dimension, where 1 is very poor
and 5 is excellent. Use exactly these five dimensions:
- Diagnostic Transparency
- Evidence Traceability
- Reasoning Confidence
- Information Completeness
- Trust Level
\end{promptbox}

The judge outputs structured JSON with 1--5 Likert scores and reasoning for each dimension. The five dimensions are defined as follows:
\begin{description}
\item[\textbf{Diagnostic Transparency}] Whether the patient can understand how the diagnosis was derived from the consultation.
\item[\textbf{Evidence Traceability}] Whether the connections between reported symptoms and the diagnosis are visible and verifiable.
\item[\textbf{Reasoning Confidence}] The patient's confidence in the system's diagnostic reasoning process.
\item[\textbf{Information Completeness}] Whether the consultation provided sufficient information for the patient to evaluate the diagnosis.
\item[\textbf{Trust Level}] Overall willingness to trust and accept the diagnostic result.
\end{description}
Under the with-KG condition, \texttt{\{CONDITION\_DESCRIPTION\}} includes a formatted description of the interactive knowledge graph visualization. Under the without-KG condition, it states that no visualization was shown.

\subsection{Cognitive Load Evaluation Prompts (RQ3.1)}
The cognitive load evaluation assesses whether structured multimodal treatment plans reduce cognitive load for non-expert users (RQ3.1). The judge model adopts the persona of a patient with limited education and no medical background.

\begin{promptbox}{Listing 6: Evaluator system prompt.}
You are an ordinary person with only middle school education and
NO medical background. You cannot read classical Chinese medical
terms. You live in a rural area. You need to understand this
treatment plan and follow it at home. Use simple everyday language
and avoid medical jargon in your reasoning.
\end{promptbox}

\begin{promptbox}{Listing 7: Evaluation user prompt template.}
You are an ordinary person with only middle school education. You
have no medical training. You cannot read classical Chinese medical
terms. You live in a rural area. You are using a health app on
your smartphone.

A doctor has given you this treatment plan. Please try to mentally
follow the instructions.

Plan Type: {PLAN_TYPE}
{MULTIMODAL_NOTE}

[PLAN CONTENT]
{PLAN_CONTENT}

Rate how well you understood each aspect (1=completely confused,
5=perfectly clear):
- Language Comprehensibility
- Preparation Clarity
- Acupoint Locatability
- Action Confidence
- Overall Cognitive Load
\end{promptbox}

The evaluator outputs structured JSON with 1--5 Likert scores and reasoning for each dimension. The five dimensions are defined as follows:
\begin{description}
\item[\textbf{Language Comprehensibility}] Whether the patient can understand the instructions.
\item[\textbf{Preparation Clarity}] Whether the patient understands how to prepare, cook, or use each item.
\item[\textbf{Acupoint Locatability}] Whether the patient can find the exact body location to press.
\item[\textbf{Action Confidence}] How confident the patient feels about following the plan correctly.
\item[\textbf{Overall Cognitive Load}] How mentally taxing it was to understand the plan (reverse scored: 1=very easy, 5=very hard; converted to 6 minus original score during analysis).
\end{description}
Plan~A is the system-generated plain-text treatment recommendation. Plan~B restructures the same content into a structured multimodal format with step-by-step guides, AI-generated herbal ingredient images, and text descriptions of 3D acupoint models and demonstration videos. \texttt{\{MULTIMODAL\_NOTE\}} describes the available visual aids for each condition.

\subsection{Evidence Credibility Evaluation Prompts (RQ3.2)}
The evidence credibility evaluation assesses whether appending references to treatment recommendations improves perceived evidence quality (RQ3.2).

\begin{promptbox}{Listing 8: Judge system prompt.}
You are an expert evaluator assessing a Traditional Chinese
Medicine (TCM) diagnostic web application's treatment advice
module.

The system generates personalized treatment plans including dietary
recommendations, herbal remedies, exercise guidance, and
acupuncture point suggestions based on TCM syndrome
differentiation.

Your task is to evaluate how well the treatment advice presentation
supports patient comprehension and trust, specifically focusing on
whether the advice appears credible and evidence-based.

Score each dimension from 1 (very poor) to 5 (excellent). Provide
chain-of-thought reasoning before each score.

Return your evaluation as JSON with dimensions array containing
name, score, and reasoning fields.
\end{promptbox}

\begin{promptbox}{Listing 9: Judge user prompt template (with references).}
Patient Profile:
- Syndrome: {SYNDROME}
- Key symptoms: {SYMPTOMS}

Treatment Advice Provided to Patient:
{ADVICE_TEXT}

References and Sources Displayed to Patient:
The application displays a 'References' section below the
treatment advice with the following cited sources:

1. {REFERENCE_TITLE}
   URL: {REFERENCE_URL}
   Relevant excerpt: "{SNIPPET}"
   Verified page content (first 2000 chars): "{FETCHED_CONTENT}"

Patients can click these links to read the original sources and
verify the recommendations. You have been provided with the actual
content fetched from each source URL to assess accessibility and
relevance.
\end{promptbox}

\begin{promptbox}{Listing 10: Judge user prompt template (without references).}
Patient Profile:
- Syndrome: {SYNDROME}
- Key symptoms: {SYMPTOMS}

Treatment Advice Provided to Patient:
{ADVICE_TEXT}
\end{promptbox}

The judge outputs structured JSON with 1--5 Likert scores and reasoning for each dimension. The five dimensions are defined as follows:
\begin{description}
\item[\textbf{Source Credibility}] How credible and trustworthy the treatment advice appears, considering whether the information seems to come from reliable medical/health sources.
\item[\textbf{Evidence Verifiability}] Whether specific claims and recommendations can be independently verified through traceable sources.
\item[\textbf{Information Confidence}] How confident a patient would feel following the treatment plan.
\item[\textbf{Comprehension Support}] Whether supplementary materials help the patient understand why specific treatments are recommended.
\item[\textbf{Overall Evidence Quality}] Overall assessment of the evidence-based quality of the treatment presentation.
\end{description}
Under the with-references condition, the system retrieves actual page content from each cited URL (truncated to the first 2,000 characters) so the judge can verify source accessibility and content relevance.

\bibliographystyle{unsrt}
\bibliography{references}

\end{document}
